# Supplementary material for: Joint Optimization of Autonomous Electric Vehicle Fleet Operations and Charging Station Siting
Source: arXiv:2107.00165 source file (2021-07-21)
Supplement: Supplementary file 1 [file appendix.tex]

%!TEX root = ../main.tex
\jvspace{-1em}
\section*{Nomenclature}
% Note: this appendix may appear empty if the glossary was not complied. See Readme for compilation instructions.
\label{app:nomenclature}
{\small
\printglossary[type=amod]
}
